# Supplementary material for: Shape-driven Coordinate Ordering for Star Glyph Sets via Reinforcement Learning
Source: arXiv:2103.02380 source file (2021-03-03)
Supplement: Supplementary file 1 [file appendix.tex]

\section*{Appendix}

% \subsection*{Neural network details}
% \label{subsec:network}

% In this section, we discuss the architecture and training of our coordinate ordering neural network in more detail.

% \noindent{\textit{a) Network architecture}}
% \subsubsection*{Network architecture}
\subsection*{Network architecture}

	Our coordinate ordering network can be divided into two components: (i) an actor network which predicts a probability distribution over the next action at any given decision step, and (ii) a critic network which estimates the reward for the given input. Figure~\ref{fig:network_structure} illustrates the architectures of these two components, which are formed from a few basic modules: 1) embedded RNN module, 2) decoder RNN module, 3) actor attention module, and 4) critic glimpse module. 
	Both the actor network and the critic network have two embedded RNN modules and a decoder RNN module. In addition, the actor network also has an actor attention module while the critic network has a critic glimpse module. 
	%We will explain the details of each module in the following sections.
	The full architectures of these modules are listed in Tables~\ref{tab:embed}, \ref{tab:rnn}, \ref{tab:actor}, and~\ref{tab:critic}. 

	%\textit{Embedded RNN module}: To handle inputs of various sizes, 1-layer gated recurrent units (GRU) are used to embed the input data into high-dimensional vectors.

	%\textit{Decoder RNN module}: a 1-layer GRU.

	%\textit{Actor attention module}: The actor attention module receives the embedded vectors from the encoder and the hidden state vector from the decoder, and then selects the output from the encoder input set according to the distribution computed by the attention mechanism. The process repeats untill all inputs are selected.
	%, which we explain in Section~\ref{subsubsec:attention}.

	% copy
	%\textit{Critic glimpse module}: The critic glimpse module receives the embedded vectors and the hidden state from the decoder RNN module, and performs $P$ steps (3 steps in our network) of computation over the hidden state $\omega_c$. Each processing step updates this hidden state by glimpsing at the embedded vectors.
	% , which we will discuss later.
	%as described in Section~\ref{subsubsec:glimpse}. 
	%The module then feeds the output of the glimpse function as input to the next processing step. The final hidden state obtained is decoded into a baseline prediction (a reward scalar) by two fully-connected layers.

% \noindent{\textit{b) Network training}}
% \subsubsection*{Network training}
\subsection*{Network training}

	We use the actor-critic training algorithm of Bello et al.~\cite{bello2017} to train our network, which is described in Algorithm~\ref{alg:training}. We parameterize the stochastic policy $\pi$ with parameters $\theta$, where $\theta$ is a vector of all trainable variables used in the actor network. The critic network is parameterized by $\theta_c$. Once a sequence of coordinates is decided, we compute the total reward and use its negative value as the reward signal.
	% loss

	In each batch, for a given input set $X_i$, our actor returns a sequence, the reward $R(\pi_i\mid X_i)$, and the probability of sampling $p(\cdot\mid X_i)$. The critic network estimates a baseline $b_i$ for the given input. The loss function of the actor network is defined as:

	\begin{equation}
	L(\theta)=\frac{1}{B}\sum_{i=1}^{B}(R(\pi_i\mid X_i)-b_i)\log\emph{p}_\theta(\pi_i\mid X_i).
	\label{eq:tap-loss}
	\end{equation}

	% copy
	The critic is trained with stochastic gradient descent on a mean squared error objective between its predictions $b_{\theta_c}(X_i)$ and the reward output by the most recent policy. The critic loss function is formulated as:

	\begin{equation}
	L(\theta_c)=\frac{1}{B}\sum_{i=1}^{B}\Arrowvert b_{\theta_c}(X_i)-R(\pi_i\mid X_i)\Arrowvert_2^2.
	\label{eq:critic-loss}
	\end{equation}

% \subsection*{Attention and Masking}

% \noindent{\textit{a) Attention Mechanism}}
% \subsubsection*{Attention Mechanism}
% \label{subsubsec:attention}
\subsection*{Attention Mechanism}

	Our network uses the same type of attention mechanism as Nazari et al.~\cite{nazari2018}.
	For each step $t$, let $ e_i=embedded(x_i)(i \le n) $ 
	be the embedded input from the encoder.
	We denote the hidden state of the decoder's RNN cell as $\omega^t$.
	Then, an alignment vector $a^t$ is computed as:
	\begin{equation}	a^t=softmax(u^t),	\label{align_vec}	\end{equation}
	where
	\begin{equation}
			u_i^t=(v_a)^Ttanh(W_a[e_i; \omega^t]), \text{ for } i = 1,2,...,N,	\label{uit}
	\end{equation}
	where ``[\ ;\ ]'' denotes the concatenation of two vectors. Then, we compute the context vector:
	\begin{equation}	c^t = \sum_{i=1}^{N}a_i^{t}e_i.	\label{cont_vec}	\end{equation}

	Combining the context vector $c^t$ and the embedded inputs $e_i$, the probability map is computed as:
	\begin{equation}	\pi(\cdot\mid e,\omega^t) = softmax(\widetilde{u}^t),	\label{prob_map} 	\end{equation}
	where
	\begin{equation}
		\widetilde{u}_i^t = 
		\begin{cases}
			-\infty, & \text{if the coordinate has been selected}, \\ 
			(v_c)^T tanh(W_c[e_i; c^{t}]), & \text{otherwise},
		\end{cases}	\label{wide_uit}
	\end{equation}
	where $v_a$, $v_c$, $W_a$, and $W_c$ are trainable variables.

	Finally, the state with maximum probability is selected to be the output $y^t$ for step $t$.

% \noindent{\textit{b) Glimpse function}}
% \subsubsection*{Glimpse function}
% \label{subsubsec:glimpse}
\subsection*{Glimpse function}

	The glimpse function was firstly proposed by Vinyals et al.~\cite{vinyals2016}. The glimpse function $G(\{e_i\}, \omega)$ takes a set of embedded vectors and a hidden state as input and outputs an obtained hidden state. The function is defined in Algorithm~\ref{alg:glimpse}, where $v_g$ and $W_g$ are trainable variables. The glimpse function can be applied multiple times on the same embedded vector set $\{e_i\}$ according to:
	\begin{equation}
		\begin{split}
			g_0&=\omega, \\
			g_k&=G(\{e_i\},g_{k-1}).
		\end{split}
	\end{equation}

\begin{figure}[!t]
    \centering
    \includegraphics[width=0.45\textwidth]{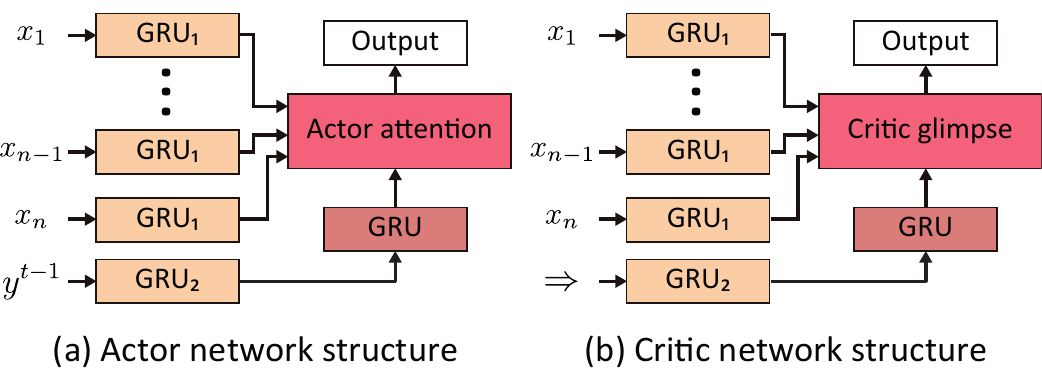}
\caption{Network structure of (a) the actor network and (b) the critic network. $n$ is the number of coordinates, and $\Rightarrow$ represents an empty initial input of the RNN module.}
\label{fig:network_structure}
\end{figure}

\begin{table}[H]%
    \caption{Embedded RNN module structure.}
    \label{tab:embed}
    \begin{minipage}{\columnwidth}
        \begin{center}        
        \noindent\begin{tabular}{l|l|l}
            \hline
            Layer & Input dim & Output dim  \\
            \hline
            GRU & $2$ & $256$ \\ 
            \hline
            \hline
            Layer & \multicolumn{1}{l}{Probability} \\
            \hline
            GRU hidden dropout & \multicolumn{1}{l}{$0.1$} \\
            \hline
        \end{tabular}

        \end{center}
    \end{minipage}
\end{table}%
\begin{table}[H]%
	\caption{Decoder RNN module structure.}
	\label{tab:rnn}
	\begin{minipage}{\columnwidth}
		\begin{center}
		\noindent\begin{tabular}{c}
			Actor
		\end{tabular}
		
		\noindent\begin{tabular}{l|l|l}
			\hline
			Layer & Input dim & Output dim  \\
            \hline
			GRU & $2$ & $256$ \\ 
            \hline
            \hline
			Layer & \multicolumn{1}{l}{Probability} \\
            \hline
			GRU hidden dropout & \multicolumn{1}{l}{$0.1$} \\
            \hline
			GRU output dropout & \multicolumn{1}{l}{$0.1$} \\
			\hline
		\end{tabular}

		\noindent\begin{tabular}{c}
			Critic
		\end{tabular}

		\noindent\begin{tabular}{l|l|l}
			\hline
			Layer & Input dim & Output dim  \\
            \hline
			GRU & $2$ & $256$ \\
            \hline
		\end{tabular}
		\end{center}
	\end{minipage}
\end{table}%
\begin{table}[H]%
	\caption{Actor attention module structure. }%\ok{What about the layers?}}
	\label{tab:actor}
	\begin{minipage}{\columnwidth}
		\begin{center}
        \begin{tabular}{l|l}
			\hline
			Parameter & Size  \\
			\hline
			$v_a$ & $1\times 256$ \\
			\hline
			$v_c$ & $1\times 256$ \\
			\hline
			$W_a$ & $256\times 512$ \\
			\hline
            $W_c$ & $256\times 512$ \\
			\hline
		\end{tabular}
		\end{center}
	\end{minipage}
\end{table}%

\begin{table}[H]%
	\caption{Critic glimpse module structure.}
	\label{tab:critic}
	\begin{minipage}{\columnwidth}
		\begin{center}
		\noindent\begin{tabular}{l|l|l}
			\hline
			Parameter & \multicolumn{1}{l}{Size} \\
			\hline
			$v_g$ & \multicolumn{1}{l}{ $1\times 256$} \\
			\hline
			$W_g$ & \multicolumn{1}{l}{ $256\times 512$} \\
			\hline
			\hline
			Layer & Input dim & Output dim  \\
			\hline
			Linear & 256 & 256 \\
			\hline
			ReLU & \multicolumn{1}{l}{-} \\
			\hline
			Linear & 256 & 1 \\
			\hline
		\end{tabular}
		
		\end{center}
	\end{minipage}
\end{table}%

	\begin{algorithm}
		\caption{Actor-critic training algorithm}  
		\label{alg:training}
		\begin{algorithmic}[1]  
			\Require  
			Training data $X$, number of training steps $T$, batch size $B$
			% \Function {A}
			% {}
			\State Initialize actor network params $\theta$
			\State Initialize critic network params $\theta_c$
			\State $t \gets 1$
			\For{$t < T$}
				\State $\pi_{i}\leftarrow p_\theta(\cdot\mid X_i)$ for $i\in\{1,...,B\}$
				\State $b_i\leftarrow b_{\theta_c}(X_i)$ for $i\in\{1,...,B\}$
				\State $L_\theta\leftarrow \frac{1}{B}\sum_{i=1}^{B}(R(\pi_i\mid X_i)-b_i)\log\emph{p}_\theta(\pi_i\mid X_i)$
				\State $L_{\theta_c}\leftarrow \frac{1}{B}\sum_{i=1}^{B}\Arrowvert b_i-R(\pi_i\mid X_i)\Arrowvert_2^2$
				\State $\theta\leftarrow $Adam($\theta,\nabla_\theta L_\theta$)
				\State $\theta_c\leftarrow $Adam($\theta_c,\nabla_{\theta_c}L_{\theta_c}$)
				\State $t \gets t+1$
			\EndFor
			% \EndFunction

		\end{algorithmic}  
	\end{algorithm}

	\begin{algorithm}
		\caption{Glimpse function}  
		\label{alg:glimpse}
		\begin{algorithmic}[1]  
			\Require
			Embedded vector set $\{e_i\}$, hidden state vector $\omega$
			\Function {Glimpse}
			{}
			\State $u_i\gets (v_g)^T tanh(W_g[e_i; \omega])$
			\State $p\gets softmax(u)$
			\State\Return $\sum_{i=1}^{N}{p_ie_i}$
			\EndFunction
		\end{algorithmic}  
	\end{algorithm}

% \noindent{\textit{c) Masking Scheme}}
% \subsubsection*{Masking Scheme}
\subsection*{Masking Scheme}

	Similarly to Nazari et al.~\cite{nazari2018}, in order to select accessible items and generate feasible solutions, we use a masking scheme which sets the log-probabilities of infeasible solutions to $-\infty$ or forces a solution if a particular condition is satisfied. For each group of data, a mask $M$ is a binary array with the same dimension as the dynamic data. $M[i]=0$ means that the $i$-th coordinate has been selected, while $M[i]=1$ means that the $i$-th coordinate is unselected. With the mask, the attention mechanism can control the probability of unselected coordinates. After the network selected a new coordinate as output, the mask is updated as:
	%\ok{unselected or can't be selected? Would we sometimes unselect acoordinate?}
	\begin{equation}
		M[i] \leftarrow
		\begin{cases}
			1,	& \text{if the } i \text{-th coordinate hasn't been selected}, \\ 
			0, & \text{otherwise}.
		\end{cases}	\label{wide_uit}
	\end{equation}
